# Supplementary material for: Improving Autonomous Driving Safety with POP: A Framework for Accurate Partially Observed Trajectory Predictions
Source: arXiv:2309.15685 source file (2024-04-05)
Supplement: Supplementary file 1 [file appendix.tex]

\appendix
\subsection{Interaction Protection Time\label{appendix:interaction_dt_model}}
\begin{equation*}
\begin{aligned}
    \Delta t_p^-(\Delta v) &= \mathbf{C_1} 
    \begin{bmatrix}
        \Delta v^4 &
        \Delta v^3 & 
        \Delta v^2 & 
        \Delta v^1 & 
        1 \\ 
    \end{bmatrix}^T, \\
    \Delta t_p^-(\Delta \theta) &= \mathbf{C_2} 
    \begin{bmatrix}
        \Delta \theta^2 & 
        \Delta \theta^1 & 
        1 \\ 
    \end{bmatrix}^T,
\end{aligned}
\end{equation*}
\noindent where $\mathbf{C_1}$ is $[3.73\times 10^{-5}, 6 \times 10^{-6}, 1.2365 \times 10^{-2}, 3.338 \times 10^{-2}, -1.165]$, $\mathbf{C_2}$ is $[-0.171, 0.095, -1.2735]$.
